# Supplementary material for: Can Large Language Models Really Improve by Self-critiquing Their Own Plans?
Source: arXiv:2310.08118 source file (2023-10-12)
Supplement: Supplementary file 1 [file 2-Appendix.tex]

\appendix
\section{Prompt for Plan Generation}
\mytcbinput{prompts/plan_gen.tex}{Plan Generation Prompt}{}{}
\section{Prompt for Plan Verification}
\mytcbinput{prompts/plan_ver.tex}{Plan Verification Prompt}{}{}
\section{Varied levels of feedback}
\subsection{Prompt for plan generation}
\mytcbinput{prompts/bp_example.tex}{Example Instance}{}{}
\subsection{Only Binary feedback}
\mytcbinput{prompts/bp_binary.tex}{GPT-4 Plan and Binary Feedback on the Plan}{}{}
\subsection{Binary + First error feedback}
\mytcbinput{prompts/bp_val.tex}{GPT-4 Plan and Binary+First Error Feedback on the Plan}{}{}
\subsection{Binary + All errors feedback}
\mytcbinput{prompts/bp_all.tex}{GPT-4 Plan and Binary+All Errors Feedback on the Plan}{}{}
